# Supplementary material for: UrbanVLP: Multi-Granularity Vision-Language Pretraining for Urban Socioeconomic Indicator Prediction
Source: arXiv:2403.16831 source file (2025-01-22)
Supplement: Supplementary file 2 [file text_calibration.tex]

\subsection{More Analysis for Text Calibration}
\label{appendix:calibration}
In our paper, we selected the state-of-the-art LMM ShareGPT4V, which demonstrates performance comparable to GPT4V in image captioning. 
In order to ascertain the efficacy of ShareGPT4V, we computed the distribution of \texttt{PerceptionScore} for descriptions generated by ShareGPT4V, as depicted in Figure \ref{fig:perceptionscore}. Notably, only less than 0.02\% of generated texts scored below 0.5, thereby evidencing the high quality of the descriptions produced.

\input{tables/compare_calibration_small}
% Noted that在这里，we propose perceptionscore 是作为生成文本质量的有力保障，同时他也印证了ShapreGPT4V的高质量和可信性。并且perceptionscore是一个plug and play, 可以广泛使用的方法，在和其他模型搭配使用的情况下，使用perceptionscore可能会过滤掉较大比例的文本，下面我们提供了一个例子说明
It is noteworthy that, \textit{we propose \texttt{PerceptionScore} as a robust guarantee for the quality of generated text, which also attests to the high quality and reliability of ShareGPT4V}. Consequently, the experimental results comparing with and without calibration in our main experiments do not adequately reflect the effectiveness of our calibration method. 
However, \texttt{PerceptionScore} is a general method that can be widely utilized across various models. When used in combination with other models, \texttt{PerceptionScore} can filter out a significant proportion of low-quality text. Next, we provide an illustrative example.

To further demonstrate the effectiveness of our method, we select mPLUG-Owl~\cite{ye2023mplug}, one of the representative LMMs compared in our paper, with the worst performance. After calibration, 15.3\% of the text with perceptionscores below 0.5 was filtered out. The results are demonstrated in Table \ref{tab:ablationresults_beijing}, which validate the effectiveness of our calibration method, and indicate that more relevant and noise-free textual information could align better with image features, leading to a more coherent and meaningful visual representation.

\begin{figure}[h]
    \centering
\includegraphics[width=0.8\columnwidth]{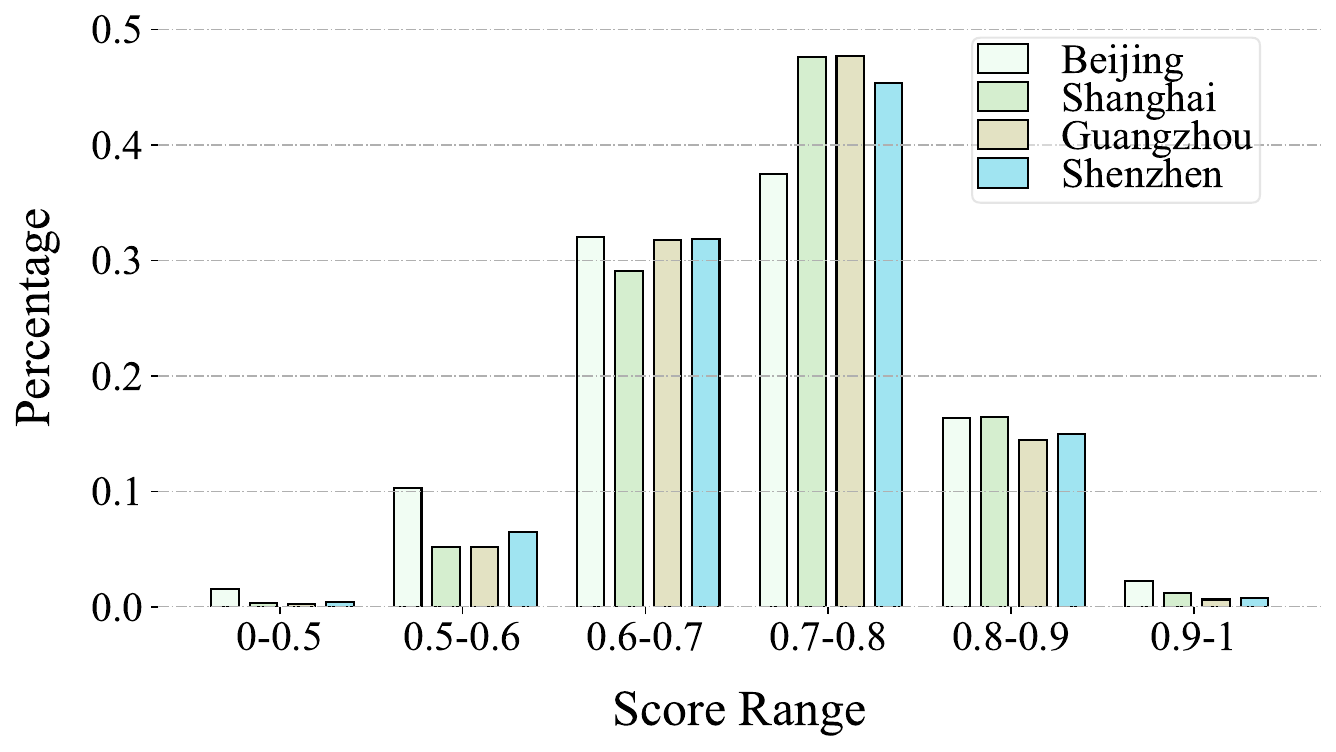}
    \caption{\texttt{PerceptionScore} distribution on $\mathtt{\dataset}$ dataset for 4 representative cities.}
    \label{fig:perceptionscore}
    \vspace{-2em}
\end{figure}
